# Supplementary material for: Getting to the Root of the Problem: Sums of Squares for Limits of Trees
Source: arXiv:2404.12838 ancillary file (2025-12-18)
Supplement: Supplementary file 1 [file README.pdf]

# My document

## Code for the paper: “Getting to the Root of the Problem: Sums of Squares for Infinite Trees”

By [Daniel Brosch](#) and [Diane Puges](#).

All code to compute the bounds, create the plots and generate some tables of the paper available at [arXiv:2404.12838](#).

Feel free to report issues with running the code at the corresponding [GitHub repository](#).

### How to run the code

The scripts automatically install all required packages and run all code in sequence, only a [Julia](#) install is required. It was only tested with Julia 1.10.3. We recommend running Julia with as many threads as your computer provides, see below. We provide a few different options:

- `runAll_lv16_Hypatia.jl`: Uses up to level 6 of the hierarchy, and uses the (Julia native) solver [Hypatia](#). Meant to check whether the code produces the expected results and plots within a couple of minutes.
- `runAll_lv18_Hypatia.jl`: Uses up to level 8 of the hierarchy, and uses the (Julia native) solver [Hypatia](#). Takes significantly longer, but gives much better bounds than level 6.
- `runAll_lv111_Mosek.jl`: Uses up to level 11 of the hierarchy, and was used to compute the bounds and plots given in the paper. It uses the commercial solver [Mosek](#) (tested with version 10.0.24). **The solver needs to be installed separately, academic licenses are available.** The code requires **significant amount of memory** (128GB should be enough) and **time** (order of multiple days on a server).

After installing Julia (and potentially Mosek), the code can be run by executing `julia -t auto runAll_lv1X_solver.jl` in a terminal. Note that on first execution relevant Julia packages will be installed, which may take a moment.

## Output

The code will generate multiple folders with output files:

- **Bounds** contains JLD2 files with all computed inducibility bounds.
- **Certificates** will contain the SOS certificates for the bounds on the inducibility graphs, and the corner of the caterpillar profiles. Only the corner certificates are given in a human-readable form, the others are given as compressed [JLD2](#) files.
- **GeneratedLatex** contains tables and lists for the paper, which we can generate automatically.
- **Models** contains computed flag SOS models (including the SDP coefficients), which speeds up further computations and can be used to verify the results.
- **Pictures** will contain the generated plots in **svg** and **pdf** formats.

## File Overview

On the upper level:

- `runAll_lv1X_solver.jl`: multiple variants of scripts executing all code, see above.

In folder `src`:

- `BlockSizeTable.jl`: Generates the table of block sizes of the optimization problems.
- `CornerCat456.jl`: Computes the corner certificate for the caterpillar profiles, and makes it rigorous.
- `DrawProfiles.jl`: Uses the computed bounds to plot the various approximations of tree profiles.
- `NonConvexity.jl`: Computes a rigorous non convexity certificate.
- `TreeInducibility.jl`: Computes bounds on the inducibility of trees.
- `TreeProductTable.jl`: Generates the table for products of small tree flags.
- `TreeProfiles.jl`: Computes the approximations of the profiles of trees.

## A note on the implementation of the flag algebra

The flag algebra itself was implemented by the authors as part of the Julia package [FlagSOS.jl](#), which this code uses. The package is designed to be easily expandable. Given appropriate functions for gluing and checking for automorphisms (implemented for trees in the file [src/FlagAlgebras/BinaryTrees.jl](#) of the FlagSOS package), the package provides all functions necessary to solve flag sums of squares problems.
